# Supplementary material for: Single artificial atoms in silicon emitting at telecom wavelengths
Source: arXiv:2001.02136 ancillary file (2020-01-07)
Supplement: Supplementary file 1 [file article_Redjem_Durand_arXiv_SI.pdf]

# Single artificial atoms in silicon emitting at telecom wavelengths
# Methods

W. Redjem[1],* A. Durand[1],* T. Herzig[2], A. Benali[3], S. Pezzagna[2], J. Meijer[2], A. Yu. Kuznetsov[4], H. S. Nguyen[5], S. Cueff[5], J.-M. Gérard[6], I. Robert-Philip[1], B. Gil[1], D. Caliste[6], P. Pochet[6], M. Abbarchi[3], V. Jacques[1], A. Dréau[1],† and G. Cassabois[1]

[1]*Laboratoire Charles Coulomb, Université de Montpellier and CNRS, 34095 Montpellier, France*

[2]*Division of Applied Quantum Systems, Felix-Bloch Institute for Solid-State Physics, University Leipzig, Linnéstraße 5, 04103 Leipzig, Germany*

[3]*CNRS, Aix-Marseille Université, Centrale Marseille, IM2NP, UMR 7334, Campus de St. Jérôme, 13397 Marseille, France*

[4]*Department of Physics, University of Oslo, NO-0316 Oslo, Norway*

[5]*Institut des Nanotechnologies de Lyon-INL, UMR CNRS 5270, CNRS, Ecole Centrale de Lyon, Ecully, France and*

[6]*Department of Physics, IRIG, Univ. Grenoble Alpes and CEA, F-38000 Grenoble, France.*

## I. SAMPLE PREPARATION.

The sample was cut from a standard commercial SOI wafer with a 220-nm thick top layer of silicon. The sample was implanted with carbon ions at 36 keV and with a fluence of $5 \times 10^{13}\,\text{cm}^{-2}$. The implantation energy has been chosen from SRIM calculations [1], to ensure that the carbon atoms stop on average at 100 nm below the sample surface. In order to heal the silicon lattice from implantation damages, a flash annealing of 20 s at 1000°C under $N_2$ atmosphere has been subsequently performed.

## II. EXPERIMENTAL SETUP.

The experimental setup consists of a home-made confocal microscope built up in a He-closed-cycle cryostat (MyCryoFirm). Optical excitation and collection of the sample are performed with a microscope objective (Olympus, LCPLN100XIR) installed inside the vacuum chamber of the cryostat. Sample photoluminescence (PL) is measured with fiber-coupled near-infrared single photon detectors (IDQuantique, ID230), featuring a quantum efficiency $\eta_{\rm det} = 10\%$ and dark counts below 50 counts/s. The filtering of the excitation laser light at 532 nm is implemented by using a dichroic mirror (Thorlabs, DMLP1000) and by coupling the PL into the single-mode optical fiber of the near-infrared detectors. No extra filtering is applied on the collected PL. The optical power indicated in the main text is measured in front of the input window of the cryostat vacuum chamber. The focal spot size of the confocal microscope is estimated to be $\simeq$ 500 nm at full width at half maximum. Experiment control and data acquisition are carried out by Python programs from the collaborative Qudi project [2].

## III. PHOTODYNAMICS.

The second-order correlation function $g^{(2)}(\tau)$ is recorded following the method described in ref. [3]. To assess the purity of isolated G-centers, this function is corrected from imperfect signal-to-noise ratio (SNR) resulting from background PL and detector dark counts on Extended Data Fig. 1a, according to the following equation [4]:

$$g^{(2)}_{\rm cor}(\tau) = \frac{g^{(2)}(\tau) - (1-\rho^2)}{\rho^2} \tag{1}$$

where $\rho$ is related to the SNR by $\rho = 1/(1 + 1/\text{SNR})$. Once corrected from environment and detection noises, the autocorrelation function at zero delay $g^{(2)}_{\rm cor}(0)$ goes to zero (Extended Data Fig. 1b), ensuring that solely a single

---

* Contributed equally to this work.
† anais.dreau@umontpellier.fr

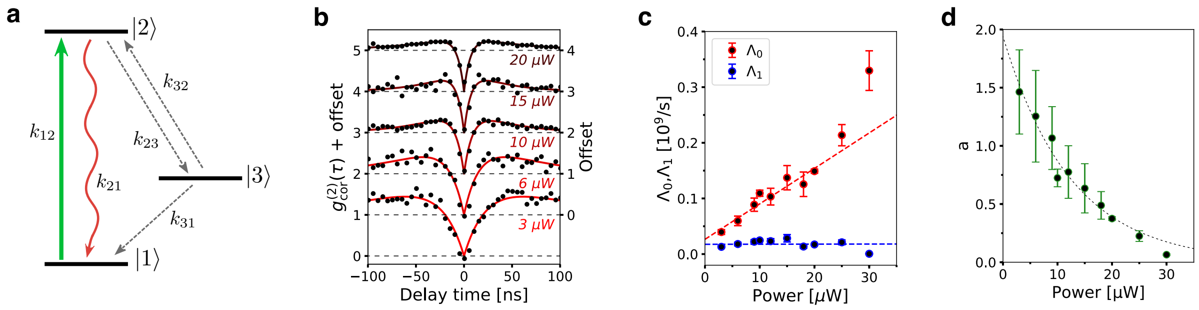


Extended Data FIG.1. **Analysis of the photodynamics of the G-center.** **a**, Simplified three-level model of the G-center under optical excitation. **b**, Second-order correlation function $g^{(2)}_{\rm cor}(\tau)$ with increasing laser excitation power (from bottom to top). Data are corrected from background counts (see Eq. 1) and fitted with equation 3. **c**, Evol -ution of the rates $\Lambda_0$ and $\Lambda_1$ with increasing optical power. The dashed lines correspond to data fitting excluding the last point at 30 $\mu$W. **d**, The bunching amplitude decreases with increasing optical power. The dotted line is a guide to the eye. Error bars represent the standard error resulting from data fitting of **b** with Python *lmfit* function.

optical transition is involved in the single-photon emission process. Note that all the data shown in the main text are not corrected from the background signal.

To simulate the photodynamics of G-centers, we consider the 3-level toy-model represented on Extended Data Fig. 1a. Once optically excited from the ground level $|1\rangle$ to the excited level $|2\rangle$, the defect can relax into its fundamental level following two paths: either through a direct radiative transition or via a non-radiative transition involving a metastable level $|3\rangle$. For this 3-level system (3LS), the $g^{(2)}_{\rm 3LS}(\tau)$ function can be expressed in terms of the population of the excited level $p_2$ following the formula $g^{(2)}_{\rm 3LS}(\tau) = p_2(\tau)/p_2(\infty)$, where $p_2(\infty)$ represents the steady-state population of level $|2\rangle$. The time evolution of the population $p_i(t)_{\{i\in[1,2,3]\}}$ can be inferred by solving the following rate equations : $d\vec{p}/dt = \mathbf{A}\vec{p}$, where $\vec{p}(t) = \{p_i(t)\}_{i\in[1,2,3]}$ and

$$\mathbf{A} = \begin{pmatrix} -k_{12} & k_{21} & k_{31} \\ k_{12} & -k_{21}-k_{23} & k_{32} \\ 0 & k_{23} & -k_{31}-k_{32} \end{pmatrix}. \tag{2}$$

The two boundary conditions are $g^{(2)}_{\rm 3LS}(0) = 0$ considering an ideal single-photon source and $g^{(2)}_{\rm 3LS}(\infty) = 1$ since all correlations are lost after a given time. Using those conditions and given that the matrix $\mathbf{A}$ has two non-zero eigenvalues, the general formula for the autocorrelation function writes as follows[33]:

$$g^{(2)}_{\rm 3LS}(\tau) = 1-(1-a)e^{-\Lambda_0\tau} + ae^{-\Lambda_1\tau}\,, \tag{3}$$

with the three parameters $a, \Lambda_0$ and $\Lambda_1$ being non-trivial functions of the effective rates $k_{ij}$ of the model[33]. In first approximation, the second term describes the antibunching effect at short time scale, while the last term dominates the bunching behaviour at long time scale.

Autocorrelation function data recorded on the single G-center presented in the main text and corrected from imperfect SNR are fitted with Equation 3 to extract the evolution of the free parameters $(a, \Lambda_0, \Lambda_1)$ with increasing optical power. In the main text, the data are not corrected from background and are fitted with the formula: $g^{(2)}(\tau) = 1-\rho^2+\rho^2\cdot g^{(2)}_{\rm 3LS}(\tau)$.

As depicted on Extended Data Fig. 1c, the rate $\Lambda_0$ associated with the antibunching increases with optical power while the other rate $\Lambda_1$ remains pretty constant. When the optical power tends to zero, the first rate $\Lambda_0$ should lead to the inverse of the excited level life time $\tau_e$. From a linear fit of the data, the value at origin gives a lifetime of $37\pm9$ ns, in good agreement with the value measured on the same center by time-resolved PL (see Fig. 3a from the main text). In a 3-level model where $k_{32}=0$, the bunching amplitude $a$ increases with optical power [5]. Here on the contrary, this parameter decreases towards zero at high optical power (Extended Data Fig. 1d). This behaviour can be qualitatively understood by the presence of a repumping rate $k_{32}$ increasing with optical power and transferring the population from the metastable level $|3\rangle$ to the excited level $|2\rangle$, likely involving transition via the conduction band (see Fig. 3c from the main text).

## IV. DFT CALCULATIONS OF THE G-CENTER STRUCTURE.

Calculations were performed with the BigDFT software [6] following the methodology described in ref. [7]. In order to further reduce the interaction between periodic images of the defect described in Figure 2a, we enlarge our supercell from 216 to 512 atoms. From the DFT results, the straight line joining the two carbon atoms is found to be close to the {111} direction. The interstitial silicon of the G-center sits in one of the three equivalent symmetry planes of the crystal containing this direction, at equal distance of the two neighboring carbons.

[1] J. F. Ziegler, Nuclear Instruments and Methods in Physics Research Section B: Beam Interactions with Materials and Atoms Proceedings of the Sixteenth International Conference on Ion Beam Analysis, **219-220**, 1027 (2004).
[2] J. M. Binder, A. Stark, N. Tomek, J. Scheuer, F. Frank, K. D. Jahnke, C. Müller, S. Schmitt, M. H. Metsch, T. Unden, T. Gehring, A. Huck, U. L. Andersen, L. J. Rogers, and F. Jelezko, SoftwareX **6**, 85 (2017).
[3] L. J. Martínez, T. Pelini, V. Waselowski, J. R. Maze, B. Gil, G. Cassabois, and V. Jacques, Physical Review B **94**, 121405 (2016).
[4] A. Beveratos, S. Kühn, R. Brouri, T. Gacoin, J.-P. Poizat, and P. Grangier, The European Physical Journal D **18**, 191 (2002).
[5] A. Beveratos, R. Brouri, J.-P. Poizat, and P. Grangier, in *Quantum Communication, Computing, and Measurement 3*, edited by P. Tombesi and O. Hirota (Springer US, Boston, MA, 2002) pp. 261–267.
[6] L. Genovese, A. Neelov, S. Goedecker, T. Deutsch, S. A. Ghasemi, A. Willand, D. Caliste, O. Zilberberg, A. Rayson, M.and Bergman, and R. Schneider, The Journal of Chemical Physics **129**, 014109 (2008).
[7] D. Timerkaeva, C. Attaccalite, G. Brenet, D. Caliste, and P. Pochet, Journal of Applied Physics **123**, 161421 (2018).
